# Supplementary material for: Microgrid management with weather-based forecasting of energy generation, consumption and prices
Source: arXiv:2107.01034 source file (2021-12-09)
Supplement: Supplementary file 1 [file appendix1.tex]

%!TEX root = ../thesis.tex
% ******************************* Thesis Appendix A ****************************

\chapter{How to install \LaTeX} 

\section*{Windows OS}

\subsection*{TeXLive package - full version}
